# Supplementary material for: DEUS: Distributed Electronic Patient File Update System
Source: arXiv:2311.14349 source file (2023-11-24)
Supplement: Supplementary file 1 [file 90_appendix.tex]

%auto-ignore
\begin{lstlisting}[language=XML, caption=HL7 v3 CDA example, label=listing-cdaV2example]
<?xml version="1.0" encoding="UTF-8"?>
<ClinicalDocument xmlns="urn:hl7-org:v3" xmlns:voc="urn:hl7-org:v3/voc"
 xmlns:xsi="http://www.w3.org/2001/XMLSchema-instance"
 templateId="2.16.840.1.113883.3.27.1776">
  <!-- CDA Header -->
  <id extension="c266" root="2.16.840.1.113883.3.933"/>
  <code code="11488-4" codeSystem="2.16.840.1.113883.6.1" displayName="Consultation note"/>
  <title>Health Clinic Consultation Note</title>
  <effectiveTime value="20000407"/>
  <setId extension="BB35" root="2.16.840.1.113883.3.933"/>
  <versionNumber value="2"/>
  ...
  <recordTarget>
    <patientRole>
      <id extension="12345" root="2.16.840.1.113883.3.933"/>
      <patientPatient>
        <name>
          <given>Henry</given><family>Levin</family>
        </name>
        <administrativeGenderCode code="M" codeSystem="2.16.840.1.113883.5.1"/>
        <birthTime value="19320924"/>
      </patientPatient>
    </patientRole>
  </recordTarget>
<!-- CDA Body -->
  <component>
    <bodyChoice>
      <StructuredBody>
        <component>
          <section>
            <code code="10164-2" codeSystem="2.16.840.1.113883.6.1" codeSystemName="LOINC"/>
            <title>History of Present Illness</title>
            <text>Henry Levin, the 7th is a 67 year old male 
			referred for further asthma management. ...</text>
          </section>
        </component>
      </StructuredBody>
    </bodyChoice>
  </component>
</ClinicalDocument>
\end{lstlisting}
